# Supplementary material for: A Diagnostic Study of Explainability Techniques for Text Classification
Source: arXiv:2009.13295 source file (2020-09-25)
Supplement: Supplementary file 1 [file appendix.tex]

\documentclass[11pt,a4paper]{article}
\usepackage[hyperref]{emnlp2020}
\usepackage{times}
\usepackage{latexsym}

\usepackage{url}
\usepackage{latexsym}
\usepackage{multirow}
\usepackage{tabularx}
\usepackage{amsmath}
\usepackage{afterpage}
\usepackage{wrapfig}
\usepackage{enumitem}
\usepackage{array}
\newcolumntype{L}{>{\raggedright\arraybackslash}m{0.97\linewidth}}
\usepackage{graphicx}       %Required
\usepackage{cleveref}       % hyperlinks
\usepackage{booktabs}       % professional-quality tables
\usepackage{amsfonts}       % blackboard math symbols
\usepackage{nicefrac}       % compact symbols for 1/2, etc.
\usepackage{microtype}      % microtypography
\usepackage{float,pdflscape}
\usepackage{xcolor}
\usepackage{tikz}
\usepackage{caption}
\usepackage{subcaption}
\usepackage{tablefootnote}
\usepackage{color, colortbl}
% this is needed to have two separate pdf files for main and supplementary material
\usepackage[nokeyprefix]{refstyle}
\usepackage{varioref}
\usepackage{xr-hyper}
\usepackage{hyperref}
    \externaldocument{acl2019}
% for the multi-line text highlight
\usepackage{soul}
\usetikzlibrary{calc}
\usetikzlibrary{decorations.pathmorphing}
\definecolor{myblue}{RGB}{204, 229, 255}
\definecolor{myred}{RGB}{255, 205, 205}
\definecolor{myyellow}{RGB}{253, 253, 153}
\definecolor{mygreen}{RGB}{179, 253, 179}

% \aclfinalcopy % Uncomment this line for the final submission
%\def\aclpaperid{***} %  Enter the acl Paper ID here

%\setlength\titlebox{5cm}
% You can expand the titlebox if you need extra space
% to show all the authors. Please do not make the titlebox
% smaller than 5cm (the original size); we will check this
% in the camera-ready version and ask you to change it back.

% Attribution definitions:

% Model Definitions

% Auxiliary Definitions

\definecolor{bad_res}{HTML}{800000}
\definecolor{gr}{HTML}{18109B}
\begin{document}

\end{document}
